# Supplementary material for: Frontrunner Jones and the Raiders of the Dark Forest: An Empirical Study of Frontrunning on the Ethereum Blockchain
Source: arXiv:2102.03347 source file (2021-06-03)
Supplement: Supplementary file 1 [file appendix.tex]

\appendix

\section{Title of appendix A}
\label{appendix:a}
